# Supplementary material for: Gaussian Process Regression Adaptive Density-Guided Approach: Towards Calculations of Potential Energy Surfaces for Larger Molecules
Source: arXiv:2303.15188 ancillary file (2023-03-27)
Supplement: Supplementary file 1 [file supplementary_material.pdf]

# – Supporting Information –

## Gaussian Process Regression Adaptive Density-Guided Approach: Towards Calculations of Potential Energy Surfaces for Larger Molecules

Denis G. Artiukhin‖[1], Ian H. Godtliebsen†[2], Gunnar Schmitz¶[3], and Ove Christiansen†[4]

‖ Institut für Chemie und Biochemie, Freie Universität Berlin, Arnimallee 22, 14195 Berlin, Germany

† Department of Chemistry, Aarhus Universitet, DK-8000 Aarhus, Denmark

¶ Lehrstuhl für Theoretische Chemie II, Ruhr-Universität Bochum, Universitätstraße 150, 44801 Bochum, Germany

Date: March 27, 2023

[1]Email: denis.artiukhin@fu-berlin.de
[2]Email: ian@chem.au.dk
[3]Email: gunnar.schmitz@rub.de
[4]Email: ove@chem.au.dk

# S1 Additional Theory Aspects

## S1.1 Data Standardization

Data standardization is carried out analogously to that from the SCIKIT-LEARN (SKLEARN) package [1,2]. In the case of feature vectors $\mathbf{x}_i = (x_{i1}, x_{i2}, \cdots, x_{id})^{\mathrm{T}}$ (in this work, minimal sets of internal coordinates; see the main text), the corresponding components $\tilde{x}_{ij}$ of standardized features $\tilde{\mathbf{x}}_i$ are given as,

$$\tilde{x}_{ij} = \frac{x_{ij} - u_j^x}{s_j^x}, \tag{1}$$

where $u_j^x$ and $s_j^x$ are constant values. If the original feature vectors $\mathbf{x}_i$ for all training points are collected in the so-called design matrix,

$$\mathbf{X} = \begin{bmatrix} \mathbf{x}_1^T \\ \mathbf{x}_2^T \\ \vdots \\ \mathbf{x}_N^T \end{bmatrix}, \tag{2}$$

then the data standardization procedure for features can be described as shifting each column $j$ of values by $u_j^x$ and subsequantly scalling it by $s_j^x$. For outputs/labels $V(\mathbf{x}_i)$ (in this work, potential energy values), a very similar expression,

$$\tilde{V}(\mathbf{x}_i) = \frac{V(\mathbf{x}_i) - u^v}{s^v}, \tag{3}$$

is adopted.

If first and second derivatives of labels with respect to changes in features are also provided in the training set, which is not the case in the current work, their components should be standardized as well. Introducing the following notations for the first and second derivative components evaluated at a position $\mathbf{x}_i$,

$$g_k(\mathbf{x}_i) = \left(\frac{\mathrm{d}V}{\mathrm{d}x_k}\right)\bigg|_{\mathbf{x}_i}, \tag{4}$$

$$h_{kl}(\mathbf{x}_i) = \left(\frac{\mathrm{d}^2V}{\mathrm{d}x_k \mathrm{d}x_l}\right)\bigg|_{\mathbf{x}_i}, \tag{5}$$

we can write expressions for standardized components $\tilde{g}_k(\mathbf{x}_i)$ and $\tilde{h}_{kl}(\mathbf{x}_i)$ as,

$$\tilde{g}_k(\mathbf{x}_i) = \frac{g_k(\mathbf{x}_i) s_k^x}{s^v}, \tag{6}$$

$$\tilde{h}_{kl}(\mathbf{x}_i) = \frac{h_{kl}(\mathbf{x}_i) s_k^x s_l^x}{s^v}, \tag{7}$$

where the scaling factors $s_k^x$ and $s^v$ are those used for scaling features and labels, respectively. Predicted labels $V(\mathbf{x}_i^*)$, their derivatives, and the corresponding feature vectors $\mathbf{x}_i^*$ can be trivially shifted/scaled back using Eqs. (1), (3), (6), and (7).

There exist several possible choices, all implemented in the MidasCpp package, for constants $u$ and $s$. The available options for $u$ include shifting by:

1. Zero (no shift),
$$\forall u_j^x = 0, \tag{8}$$
$$u^v = 0. \tag{9}$$

2. Mean,
$$u_j^x = \frac{1}{N} \sum_i^N x_{ij}, \tag{10}$$
$$u^v = \frac{1}{N} \sum_i^N V(\mathbf{x}_i). \tag{11}$$

3. Mid-range (also known as mid-extreme),
$$u_j^x = \frac{\max_i(x_{ij}) + \min_i(x_{ij})}{2}, \tag{12}$$
$$u^v = \frac{\max_i(V(\mathbf{x}_i)) + \min_i(V(\mathbf{x}_i))}{2}, \tag{13}$$
where maximal and minimal values are searched for $x_{ij}$ or $V(\mathbf{x}_i)$ varying index $i$.

The available options for $s$ include scaling by:

1. One (no scaling),
$$\forall s_j^x = 1, \tag{14}$$
$$s^v = 1. \tag{15}$$

2. Population variance,
$$s_j^x = \frac{1}{N} \sum_i^N \left[ x_{ij} - \frac{1}{N} \sum_a^N x_{aj} \right]^2, \tag{16}$$
$$s^v = \frac{1}{N} \sum_i^N \left[ V(\mathbf{x}_i) - \frac{1}{N} \sum_a^N V(\mathbf{x}_a) \right]^2. \tag{17}$$

3. Sample variance,

$$s_j^x = \frac{1}{N-1} \sum_i^N \left[ x_{ij} - \frac{1}{N} \sum_a^N x_{aj} \right]^2, \tag{18}$$

$$s^v = \frac{1}{N-1} \sum_i^N \left[ V(\mathbf{x}_i) - \frac{1}{N} \sum_a^N V(\mathbf{x}_a) \right]^2. \tag{19}$$

4. Population standard deviation,

$$s_j^x = \sqrt{\frac{1}{N} \sum_i^N \left[ x_{ij} - \frac{1}{N} \sum_a^N x_{aj} \right]^2}, \tag{20}$$

$$s^v = \sqrt{\frac{1}{N} \sum_i^N \left[ V(\mathbf{x}_i) - \frac{1}{N} \sum_a^N V(\mathbf{x}_a) \right]^2}. \tag{21}$$

5. Sample standard deviation,

$$s_j^x = \sqrt{\frac{1}{N-1} \sum_i^N \left[ x_{ij} - \frac{1}{N} \sum_a^N x_{aj} \right]^2}, \tag{22}$$

$$s^v = \sqrt{\frac{1}{N-1} \sum_i^N \left[ V(\mathbf{x}_i) - \frac{1}{N} \sum_a^N V(\mathbf{x}_a) \right]^2}. \tag{23}$$

6. Absolute maximal value,

$$s_j^x = \max_i(|x_{ij}|), \tag{24}$$

$$s^v = \max_i(|V(\mathbf{x}_i)|), \tag{25}$$

where maximal values are searched for $|x_{ij}|$ or $|V(\mathbf{x}_i)|$ varying index $i$.

Because scaling and shifting could be carried out independently and separately for labels and feature vectors, different combinations of options could be applied. For example, features could be shifted by their mean values and scaled by population standard deviations, whereas labels are not shifted but scaled by their sample variance. Additionally, calculations of shifting and scaling factors, as described above, could be performed for the interquartile range of data points (difference between the 75th and 25th percentiles of the data) as opposed to calculations based on the whole dataset.

## S1.2 Initial Guesses for Hyperparameters

In addition to the option of using user-defined hyperparameters, we also implemented two initial guesses for hyperparameter optimization. These include:

1. Moment-based initialization [3], where the population standard deviation of individual features and population variance of labels are used as guesses for characteristic length-scale parameters $l_j$ and the signal variance $\sigma_f^2$, respectively, i.e.,

$$l_j = \sqrt{\frac{1}{N}\sum_i^N \left[\tilde{x}_{ij} - \frac{1}{N}\sum_a^N \tilde{x}_{aj}\right]^2}, \tag{26}$$

$$\sigma_f^2 = \frac{1}{N}\sum_i^N \left[\tilde{V}(\mathbf{x}_i) - \frac{1}{N}\sum_a^N \tilde{V}(\mathbf{x}_a)\right]^2 . \tag{27}$$

Note that standardized data enters Eqs. (26) and (27) as denoted by the tilde sign. If a single characteristic length-scale parameters $l$ is employed, it is computed by averaging $l_j$ from Eq. (26) such that,

$$l = \frac{1}{M}\sum_{j=1}^M l_j, \tag{28}$$

where $M$ is the number of parameters $l_j$ (or, in this work, the number of degrees of freedom).

2. Distance-based initialization [4], where distances between data points in the training set are employed. To that end, each $j$th column of the design matrix [see Eq. (2)] with standardized elements $\tilde{x}_{ij}$ is sorted in ascending order resulting in elements $\tilde{x}_{ij}^{\text{sort}}$. Permutations used for sorting $j$th columns are then applied to the vector of labels with elements $\tilde{V}(\mathbf{x}_i)$ to form the corresponding vectors $\tilde{\mathbf{v}}^j$. Distances between data points are subsequently represented by

$$d_j^x = \frac{1}{k_j^x}\sum_{i=1}^{N-1} |\tilde{x}_{ij}^{\text{sort}} - \tilde{x}_{(i+1)j}^{\text{sort}}| \tag{29}$$

and

$$d_j^v = \frac{1}{k_j^v}\sum_{i=1}^{N-1} |(\mathbf{v}^j)_i - (\mathbf{v}^j)_{i+1}|, \tag{30}$$

where $k_j^x$ and $k_j^v$ are the numbers of instances with $\tilde{x}_{ij}^{\text{sort}} \neq \tilde{x}_{(i+1)j}^{\text{sort}}$ and $(\mathbf{v}^j)_i \neq (\mathbf{v}^j)_{i+1}$, respectively, and $(\mathbf{v}^j)_i$ is the $i$th component of a vector $\mathbf{v}^j$. The initial guess for the

signal variance $\sigma_f^2$ is then given as the average over all $d_j^v$,

$$\sigma_f^2 = \frac{1}{M} \sum_{j=1}^{M} d_j^v. \tag{31}$$

For characteristic length-scale parameters $l_j$, either the individual components $d_j^x$ or their average could be used, i.e.,

$$l_j = d_j^x \tag{32}$$

or

$$\forall l_j = \frac{1}{M} \sum_{a=1}^{M} d_a^x. \tag{33}$$

If a single hyperparameter $l$ is adopted, the average value from Eq. (33) is assigned to it.

## S2 Reference ADGA-2M Computations

Table S1: ADGA-2M computations for water. Results for different ADGA convergence thresholds ($\epsilon_{\mathrm{rel}}$, $\epsilon_{\mathrm{abs}}$, and $\epsilon_{\rho}$) are shown. Deviations (in $\mathrm{cm}^{-1}$) are given with respect to the most accurate ADGA calculation presented in the last column. Sets of thresholds employed for production level computations in the main text are highlighted in gray.

| $\log_{10} \epsilon_{\mathrm{rel}}$ | −2 | −2 | −3 | −2 | −2 | −3 | −2 | −3 | −2 | −3 |
|---|---|---|---|---|---|---|---|---|---|---|
| $\log_{10} \epsilon_{\mathrm{abs}}$ | −3 | −3 | −3 | −4 | −4 | −4 | −5 | −5 | −6 | −6 |
| $\log_{10} \epsilon_{\rho}$ | −3 | −4 | −4 | −3 | −4 | −4 | −3 | −3 | −3 | −4 |
| MaxD | −3.59 | −3.96 | −3.96 | −0.00 | 0.06 | −0.07 | 0.02 | 0.03 | −0.01 | – |
| MinD | −7.25 | −9.65 | −9.65 | −0.50 | −0.86 | −0.42 | −0.10 | −0.31 | −0.10 | – |
| RMSD | 5.62 | 6.56 | 6.56 | 0.34 | 0.50 | 0.26 | 0.07 | 0.22 | 0.07 | – |
| No. SPs | 68 | 69 | 75 | 237 | 280 | 404 | 536 | 841 | 751 | 2086 |

Table S2: ADGA-2M computations for formaldehyde. Results for different ADGA convergence thresholds ($\epsilon_{\mathrm{rel}}$, $\epsilon_{\mathrm{abs}}$, and $\epsilon_{\rho}$) are shown. Deviations (in $\mathrm{cm}^{-1}$) are given with respect to the most accurate ADGA calculation presented in the last column. Sets of thresholds employed for production level computations in the main text are highlighted in gray.

| $\log_{10} \epsilon_{\mathrm{rel}}$ | −2 | −2 | −3 | −2 | −2 | −3 | −2 | −3 | −2 | −3 |
|---|---|---|---|---|---|---|---|---|---|---|
| $\log_{10} \epsilon_{\mathrm{abs}}$ | −3 | −3 | −3 | −4 | −4 | −4 | −5 | −5 | −6 | −6 |
| $\log_{10} \epsilon_{\rho}$ | −3 | −4 | −4 | −3 | −4 | −4 | −3 | −3 | −3 | −4 |
| MaxD | 9.16 | 8.39 | 8.39 | 4.85 | 6.01 | 6.02 | 0.06 | 0.07 | 0.04 | – |
| MinD | −17.25 | −19.61 | −19.59 | −0.60 | −0.07 | −0.12 | −0.40 | −0.62 | −0.45 | – |
| RMSD | 10.40 | 11.11 | 11.10 | 2.95 | 4.28 | 4.29 | 0.22 | 0.33 | 0.25 | – |
| No. SPs | 134 | 134 | 145 | 459 | 457 | 596 | 1812 | 2766 | 2741 | 6511 |

Table S3: ADGA-2M computations for ethylene. Results for different ADGA convergence thresholds ($\epsilon_{\text{rel}}$, $\epsilon_{\text{abs}}$, and $\epsilon_{\rho}$) are shown. Deviations (in $\text{cm}^{-1}$) are given with respect to the most accurate ADGA calculation presented in the last column. Sets of thresholds employed for production level computations in the main text are highlighted in gray.

| | | | | | | | | | | |
|---|---|---|---|---|---|---|---|---|---|---|
| $\log_{10}\epsilon_{\text{rel}}$ | −2 | −2 | −3 | −2 | −2 | −3 | −2 | −3 | −2 | −3 |
| $\log_{10}\epsilon_{\text{abs}}$ | −3 | −3 | −3 | −4 | −4 | −4 | −5 | −5 | −6 | −6 |
| $\log_{10}\epsilon_{\rho}$ | −3 | −4 | −4 | −3 | −4 | −4 | −3 | −3 | −3 | −4 |
| MaxD | 23.35 | 25.57 | 25.57 | 19.49 | 25.87 | 25.87 | 0.87 | 0.87 | 0.36 | – |
| MinD | −19.51 | −21.88 | −21.89 | −1.60 | 0.34 | 0.36 | −0.18 | −0.16 | −0.20 | – |
| RMSD | 16.43 | 18.96 | 18.96 | 10.04 | 14.09 | 14.09 | 0.37 | 0.37 | 0.14 | – |
| No. SPs | 415 | 414 | 436 | 1346 | 1292 | 1681 | 4145 | 9616 | 6306 | 17501 |

Table S4: ADGA-2M computations for imidiazole. Results for different ADGA convergence thresholds ($\epsilon_{\text{rel}}$, $\epsilon_{\text{abs}}$, and $\epsilon_{\rho}$) are shown. Deviations (in $\text{cm}^{-1}$) are given with respect to the most accurate ADGA calculation presented in the last column. Sets of thresholds employed for production level computations in the main text are highlighted in gray.

| | | | | | | | | | | |
|---|---|---|---|---|---|---|---|---|---|---|
| $\log_{10}\epsilon_{\text{rel}}$ | −2 | −2 | −3 | −2 | −2 | −3 | −2 | −3 | −2 | −3 |
| $\log_{10}\epsilon_{\text{abs}}$ | −3 | −3 | −3 | −4 | −4 | −4 | −5 | −5 | −6 | −6 |
| $\log_{10}\epsilon_{\rho}$ | −3 | −4 | −4 | −3 | −4 | −4 | −3 | −3 | −3 | −4 |
| MaxD | 98.77 | 46.11 | 46.11 | 33.07 | 46.19 | 46.17 | 1.22 | 1.22 | 0.15 | – |
| MinD | −41.85 | −140.22 | −140.23 | 1.12 | 0.60 | 0.55 | −1.73 | −1.73 | −0.44 | – |
| RMSD | 47.91 | 47.65 | 47.65 | 14.97 | 18.82 | 18.83 | 0.67 | 0.67 | 0.13 | – |
| No. SPs | 1106 | 1105 | 1125 | 3324 | 3319 | 3480 | 17105 | 22609 | 39297 | 85446 |

Table S5: ADGA-2M computations for pyrimidine. Results for different ADGA convergence thresholds ($\epsilon_{\text{rel}}$, $\epsilon_{\text{abs}}$, and $\epsilon_\rho$) are shown. Deviations (in $\text{cm}^{-1}$) are given with respect to the most accurate ADGA calculation presented in the last column. Sets of thresholds employed for production level computations in the main text are highlighted in gray.

| | | | | | | | | | | |
|---|---|---|---|---|---|---|---|---|---|---|
| $\log_{10} \epsilon_{\text{rel}}$ | −2 | −2 | −3 | −2 | −2 | −3 | −2 | −3 | −2 | −3 |
| $\log_{10} \epsilon_{\text{abs}}$ | −3 | −3 | −3 | −4 | −4 | −4 | −5 | −5 | −6 | −6 |
| $\log_{10} \epsilon_\rho$ | −3 | −4 | −4 | −3 | −4 | −4 | −3 | −3 | −3 | −4 |
| MaxD | 97.25 | 72.50 | 72.52 | 16.42 | 21.44 | 21.42 | 1.54 | 1.55 | 0.16 | – |
| MinD | −124.60 | −105.81 | −105.81 | −3.34 | −5.13 | −5.13 | −1.50 | −1.52 | −0.29 | – |
| RMSD | 54.89 | 49.12 | 49.14 | 8.09 | 10.31 | 10.32 | 0.80 | 0.80 | 0.09 | – |
| No. SPs | 1352 | 1355 | 1385 | 2939 | 3045 | 3323 | 16022 | 20756 | 33836 | 75993 |

# S3 Optimal GPR-ADGA Thresholds

Table S6: GPR-ADGA-2M computations for water. Results for different GPR-ADGA thresholds ($T_\Omega$ and $\sigma_N^2$) are shown. ADGA criteria used are $\epsilon_{\text{rel}} = 1.0 \times 10^{-2}$, $\epsilon_{\text{abs}} = 1.0 \times 10^{-5}$, and $\epsilon_\rho = 1.0 \times 10^{-3}$. Deviations (in $\text{cm}^{-1}$) are calculated with respect to the ADGA-2M calculation employing same criteria. Sets of thresholds employed for production level computations in the main text are highlighted in gray.

| $\log_{10} T_\Omega$ | $\log_{10} \sigma_N^2$ | −7 | −8 | −9 | −10 | −11 | −12 | −13 | −14 |
|---|---|---|---|---|---|---|---|---|---|
| −7 | MaxD | 3.04 | 14.43 | 18.18 | 3.58 | 3.60 | 3.60 | 3.59 | 3.59 |
| | MinD | −14.07 | −8.21 | −0.19 | −0.14 | −0.14 | −0.14 | −0.14 | −0.14 |
| | RMSD | 8.39 | 9.59 | 10.83 | 2.19 | 2.20 | 2.20 | 2.20 | 2.20 |
| | ML iter. | 8 | 8 | 9 | 10 | 10 | 10 | 10 | 10 |
| | No. SPs | 102 | 103 | 112 | 113 | 113 | 113 | 113 | 113 |
| −8 | MaxD | −1.01 | 0.44 | 1.22 | 1.72 | 1.65 | 1.68 | 1.69 | 1.65 |
| | MinD | −3.36 | −1.05 | −0.14 | −0.09 | −0.11 | −0.09 | −0.08 | −0.10 |
| | RMSD | 2.13 | 0.73 | 0.72 | 1.02 | 0.98 | 0.99 | 1.00 | 0.98 |
| | ML iter. | 9 | 10 | 10 | 10 | 10 | 10 | 10 | 10 |
| | No. SPs | 112 | 126 | 124 | 129 | 130 | 130 | 130 | 130 |
| −9 | MaxD | −0.48 | 0.20 | 0.54 | 1.06 | 1.06 | 1.05 | 1.05 | 1.05 |
| | MinD | −2.62 | −1.22 | −0.94 | 0.09 | 0.07 | 0.07 | 0.07 | 0.07 |
| | RMSD | 1.59 | 0.72 | 0.63 | 0.67 | 0.67 | 0.67 | 0.67 | 0.67 |
| | ML iter. | 16 | 12 | 14 | 13 | 13 | 13 | 13 | 13 |
| | No. SPs | 209 | 140 | 157 | 159 | 159 | 159 | 159 | 159 |
| −10 | MaxD | 0.70 | 0.22 | 0.21 | 0.21 | 0.03 | 0.03 | 0.03 | 0.03 |
| | MinD | −0.50 | −0.43 | −0.68 | −0.56 | −0.56 | −0.57 | −0.57 | −0.57 |
| | RMSD | 0.50 | 0.28 | 0.43 | 0.35 | 0.35 | 0.35 | 0.35 | 0.35 |
| | ML iter. | 41 | 20 | 15 | 17 | 17 | 17 | 17 | 17 |
| | No. SPs | 552 | 248 | 185 | 209 | 211 | 211 | 211 | 211 |
| −11 | MaxD | 0.85 | 0.01 | −0.07 | 0.28 | 0.11 | 0.05 | 0.04 | 0.04 |
| | MinD | −0.27 | −0.20 | −0.83 | −0.03 | 0.01 | −0.98 | −1.15 | −1.15 |
| | RMSD | 0.52 | 0.15 | 0.52 | 0.16 | 0.09 | 0.58 | 0.71 | 0.71 |
| | ML iter. | 50 | 46 | 24 | 27 | 25 | 20 | 20 | 20 |
| | No. SPs | 633 | 560 | 302 | 301 | 296 | 246 | 250 | 250 |
| −12 | MaxD | 0.85 | −0.01 | 0.03 | 0.08 | 0.00 | 0.00 | 0.00 | 0.00 |
| | MinD | −0.27 | −0.18 | −0.08 | −0.03 | −0.03 | −0.05 | −0.05 | −0.05 |
| | RMSD | 0.52 | 0.12 | 0.05 | 0.05 | 0.02 | 0.03 | 0.03 | 0.03 |
| | ML iter. | 50 | 50 | 50 | 37 | 31 | 30 | 30 | 30 |
| | No. SPs | 633 | 583 | 564 | 443 | 356 | 364 | 364 | 364 |
| −13 | MaxD | 0.85 | −0.01 | 0.02 | 0.03 | 0.00 | 0.01 | 0.01 | 0.00 |
| | MinD | −0.27 | −0.18 | −0.08 | 0.00 | 0.00 | 0.00 | 0.00 | 0.00 |
| | RMSD | 0.52 | 0.12 | 0.05 | 0.02 | 0.00 | 0.00 | 0.00 | 0.00 |
| | ML iter. | 50 | 50 | 50 | 50 | 41 | 42 | 40 | 40 |
| | No. SPs | 633 | 583 | 565 | 567 | 492 | 520 | 461 | 461 |
| −14 | MaxD | 0.85 | −0.01 | 0.02 | 0.03 | 0.01 | 0.00 | 0.00 | 0.00 |
| | MinD | −0.27 | −0.18 | −0.08 | 0.00 | 0.00 | 0.00 | 0.00 | 0.00 |
| | RMSD | 0.52 | 0.12 | 0.05 | 0.02 | 0.00 | 0.00 | 0.00 | 0.00 |
| | ML iter. | 50 | 50 | 50 | 50 | 50 | 49 | 40 | 40 |
| | No. SPs | 633 | 583 | 565 | 567 | 568 | 545 | 471 | 469 |

# S4 Stopping Hyperparameter Optimization

Table S7: GPR-ADGA-2M computations for water using different criteria for stopping hyperparameter optimization. ADGA criteria used are $\epsilon_{\text{rel}} = 1.0 \times 10^{-2}$, $\epsilon_{\text{abs}} = 1.0 \times 10^{-5}$, and $\epsilon_{\rho} = 1.0 \times 10^{-3}$. Deviations (in $\text{cm}^{-1}$) are calculated with respect to the reference ADGA-2M calculation (with 536 SPs) employing same criteria. Results for the threshold employed for production level computations in the main text are highlighted in gray.

| SPs per 2M cut | $\sigma_N^2$, $T_\Omega$ | $1.0 \times 10^{-8}$ | $1.0 \times 10^{-9}$ | $1.0 \times 10^{-10}$ | $1.0 \times 10^{-11}$ |
|---|---|---|---|---|---|
| 0 | MaxD | 22.88 | 1.01 | 0.03 | 0.61 |
| | MinD | −37.84 | −0.50 | −0.99 | −2.71 |
| | RMSD | 25.55 | 0.65 | 0.60 | 1.61 |
| | No. SPs | 102 | 121 | 144 | 168 |
| 5 | MaxD | 1.12 | 0.10 | 0.03 | 0.05 |
| | MinD | −11.72 | −2.52 | −0.83 | −0.31 |
| | RMSD | 6.81 | 1.53 | 0.67 | 0.23 |
| | No. SPs | 153 | 190 | 212 | 238 |
| 10 | MaxD | 0.69 | 2.18 | −0.08 | 0.02 |
| | MinD | 0.16 | −4.47 | −1.92 | −0.08 |
| | RMSD | 0.44 | 2.88 | 1.53 | 0.05 |
| | No. SPs | 136 | 163 | 190 | 213 |
| 15 | MaxD | −0.39 | 1.10 | 0.20 | 0.60 |
| | MinD | −2.51 | 0.12 | −1.82 | −1.10 |
| | RMSD | 1.66 | 0.67 | 1.06 | 0.72 |
| | No. SPs | 112 | 133 | 167 | 173 |
| 20 | MaxD | 2.18 | 0.46 | 0.53 | 0.10 |
| | MinD | 0.66 | −0.42 | −1.68 | −0.40 |
| | RMSD | 1.43 | 0.36 | 1.02 | 0.30 |
| | No. SPs | 127 | 147 | 171 | 186 |
| 25 | MaxD | 1.22 | 0.38 | 0.07 | 0.06 |
| | MinD | 0.19 | 0.16 | −1.03 | −0.73 |
| | RMSD | 0.74 | 0.27 | 0.71 | 0.42 |
| | No. SPs | 125 | 141 | 166 | 172 |
| 30 | MaxD | 0.69 | 0.41 | 0.53 | −0.07 |
| | MinD | −1.48 | −0.05 | 0.04 | −0.63 |
| | RMSD | 0.99 | 0.25 | 0.40 | 0.37 |
| | No. SPs | 121 | 136 | 156 | 170 |

Table S8: GPR-ADGA-2M computations for formaldehyde using different criteria for stopping hyperparameter optimization. ADGA criteria used are $\epsilon_{\text{rel}} = 1.0 \times 10^{-2}$, $\epsilon_{\text{abs}} = 1.0 \times 10^{-5}$, and $\epsilon_{\rho} = 1.0 \times 10^{-3}$. Deviations (in $\text{cm}^{-1}$) are calculated with respect to the reference ADGA-2M calculation (with 1812 SPs) employing same criteria. Results for the threshold employed for production level computations in the main text are highlighted in gray.

| SPs per 2M cut | $\sigma_N^2$, $T_\Omega$ | $1.0 \times 10^{-8}$ | $1.0 \times 10^{-9}$ | $1.0 \times 10^{-10}$ | $1.0 \times 10^{-11}$ |
|---|---|---|---|---|---|
| 0 | MaxD | 0.73 | 0.12 | 0.06 | 0.04 |
| | MinD | 0.25 | −0.06 | −0.05 | −0.16 |
| | RMSD | 0.47 | 0.07 | 0.04 | 0.08 |
| | No. SPs | 908 | 1077 | 1241 | 1393 |
| 5 | MaxD | 0.32 | 0.32 | 0.12 | 0.00 |
| | MinD | −7.16 | −0.37 | −0.51 | −0.14 |
| | RMSD | 2.98 | 0.25 | 0.22 | 0.09 |
| | No. SPs | 683 | 828 | 935 | 1074 |
| 10 | MaxD | 0.14 | 0.36 | 0.19 | 0.13 |
| | MinD | −2.14 | −4.99 | 0.05 | −0.72 |
| | RMSD | 0.88 | 2.05 | 0.13 | 0.37 |
| | No. SPs | 609 | 741 | 855 | 965 |
| 15 | MaxD | 0.59 | 0.59 | 0.32 | 0.13 |
| | MinD | 0.00 | −0.11 | −1.51 | −0.76 |
| | RMSD | 0.31 | 0.25 | 0.63 | 0.38 |
| | No. SPs | 539 | 636 | 732 | 930 |
| 20 | MaxD | 1.69 | 1.14 | 0.34 | 0.51 |
| | MinD | 0.13 | −0.02 | −0.42 | −0.04 |
| | RMSD | 0.73 | 0.49 | 0.25 | 0.21 |
| | No. SPs | 498 | 594 | 712 | 840 |
| 25 | MaxD | 5.61 | 1.26 | 0.15 | 0.32 |
| | MinD | −0.02 | −0.06 | −0.17 | −0.13 |
| | RMSD | 2.34 | 0.56 | 0.10 | 0.16 |
| | No. SPs | 478 | 567 | 668 | 801 |
| 30 | MaxD | 4.87 | 0.67 | 0.36 | 0.52 |
| | MinD | −0.13 | −0.02 | −1.45 | 0.02 |
| | RMSD | 2.03 | 0.33 | 0.63 | 0.22 |
| | No. SPs | 466 | 643 | 758 | 858 |

Table S9: GPR-ADGA-2M computations for ethylene using different criteria for stopping hyperparameter optimization. ADGA criteria used are $\epsilon_{\text{rel}} = 1.0 \times 10^{-2}$, $\epsilon_{\text{abs}} = 1.0 \times 10^{-5}$, and $\epsilon_\rho = 1.0 \times 10^{-3}$. Deviations (in $\text{cm}^{-1}$) are calculated with respect to the reference ADGA-2M calculation (with 4145 SPs) employing same criteria. Results for the threshold employed for production level computations in the main text are highlighted in gray.

| SPs per 2M cut | $\sigma_N^2$, $T_\Omega$ | $1.0 \times 10^{-8}$ | $1.0 \times 10^{-9}$ | $1.0 \times 10^{-10}$ | $1.0 \times 10^{-11}$ |
|---|---|---|---|---|---|
| 0 | MaxD | 1.66 | 1.67 | 1.81 | 0.27 |
| | MinD | −3.07 | −3.10 | 0.28 | −0.42 |
| | RMSD | 2.02 | 1.46 | 0.83 | 0.19 |
| | No. SPs | 1251 | 1391 | 1796 | 2279 |
| 5 | MaxD | 10.08 | 5.70 | 0.29 | 0.11 |
| | MinD | 2.42 | 1.37 | −0.67 | −1.16 |
| | RMSD | 5.73 | 2.97 | 0.30 | 0.43 |
| | No. SPs | 1698 | 2123 | 2542 | 2441 |
| 10 | MaxD | 4.22 | 3.11 | 0.48 | −0.03 |
| | MinD | −0.91 | 0.27 | −0.20 | −0.51 |
| | RMSD | 2.14 | 1.81 | 0.21 | 0.34 |
| | No. SPs | 1503 | 1727 | 2086 | 2334 |
| 15 | MaxD | 1.92 | 3.16 | 0.38 | −0.10 |
| | MinD | −1.55 | 0.30 | −0.30 | −1.00 |
| | RMSD | 0.91 | 1.81 | 0.19 | 0.40 |
| | No. SPs | 1374 | 1790 | 2148 | 2418 |
| 20 | MaxD | 1.59 | 2.03 | 0.44 | −0.17 |
| | MinD | −1.81 | 0.04 | −0.26 | −1.13 |
| | RMSD | 0.87 | 1.25 | 0.20 | 0.45 |
| | No. SPs | 1379 | 1803 | 2191 | 2501 |
| 25 | MaxD | 1.34 | 2.20 | 0.03 | 0.14 |
| | MinD | −1.80 | 0.00 | −0.33 | −0.75 |
| | RMSD | 0.80 | 1.33 | 0.15 | 0.29 |
| | No. SPs | 1389 | 1780 | 2135 | 2813 |
| 30 | MaxD | 1.34 | 2.07 | 0.38 | 0.07 |
| | MinD | −1.80 | 0.03 | −0.30 | −0.72 |
| | RMSD | 0.80 | 1.34 | 0.18 | 0.26 |
| | No. SPs | 1389 | 1769 | 2190 | 2869 |

Table S10: GPR-ADGA-2M computations for imidazole using different criteria for stopping hyperparameter optimization. ADGA criteria used are $\epsilon_{\text{rel}} = 1.0 \times 10^{-2}$, $\epsilon_{\text{abs}} = 1.0 \times 10^{-5}$, and $\epsilon_{\rho} = 1.0 \times 10^{-3}$. Deviations (in $\text{cm}^{-1}$) are calculated with respect to the reference ADGA-2M calculation (with 17105 SPs) employing same criteria. Results for the threshold employed for production level computations in the main text are highlighted in gray.

| SPs per 2M cut | $\sigma_N^2$, $T_\Omega$ | $1.0 \times 10^{-8}$ | $1.0 \times 10^{-9}$ | $1.0 \times 10^{-10}$ | $1.0 \times 10^{-11}$ |
|---|---|---|---|---|---|
| 0 | MaxD | 7.75 | −1.11 | 1.84 | 0.59 |
| | MinD | −6.26 | −7.21 | −2.05 | −1.07 |
| | RMSD | 3.32 | 3.22 | 1.00 | 0.35 |
| | No. SPs | 8194 | 9610 | 10850 | 12092 |
| 5 | MaxD | 1.12 | 0.39 | −0.23 | −0.03 |
| | MinD | −7.05 | −12.91 | −3.90 | −1.55 |
| | RMSD | 3.41 | 4.56 | 1.42 | 0.53 |
| | No. SPs | 9961 | 11360 | 13014 | 14258 |
| 10 | MaxD | 1.97 | 2.66 | −0.42 | 0.36 |
| | MinD | −8.14 | −2.86 | −2.04 | −1.38 |
| | RMSD | 3.76 | 1.52 | 1.00 | 0.44 |
| | No. SPs | 9828 | 14313 | 15402 | 16728 |
| 15 | MaxD | 6.18 | 0.57 | −0.25 | 0.09 |
| | MinD | 1.44 | −0.99 | −1.89 | −1.21 |
| | RMSD | 3.18 | 0.46 | 0.93 | 0.35 |
| | No. SPs | 6065 | 7885 | 13097 | 14755 |
| 20 | MaxD | 5.58 | 0.92 | 0.32 | 0.31 |
| | MinD | 1.11 | −0.21 | −1.09 | −1.05 |
| | RMSD | 2.60 | 0.53 | 0.48 | 0.33 |
| | No. SPs | 6102 | 7561 | 12156 | 14328 |
| 25 | MaxD | 4.90 | 0.96 | 0.32 | 0.51 |
| | MinD | 0.70 | −0.07 | −1.33 | −1.07 |
| | RMSD | 2.10 | 0.54 | 0.68 | 0.33 |
| | No. SPs | 5926 | 7452 | 8304 | 14007 |
| 30 | MaxD | 4.77 | 1.19 | 0.67 | 0.46 |
| | MinD | −0.46 | −0.15 | −1.26 | −0.97 |
| | RMSD | 2.04 | 0.65 | 0.63 | 0.37 |
| | No. SPs | 5882 | 7250 | 8289 | 13420 |

Table S11: GPR-ADGA-2M computations for pyrimidine using different criteria for stopping hyperparameter optimization. ADGA criteria used are $\epsilon_{\text{rel}} = 1.0 \times 10^{-2}$, $\epsilon_{\text{abs}} = 1.0 \times 10^{-5}$, and $\epsilon_{\rho} = 1.0 \times 10^{-3}$. Deviations (in $\text{cm}^{-1}$) are calculated with respect to the reference ADGA-2M calculation (with 16022 SPs) employing same criteria. Results for the threshold employed for production level computations in the main text are highlighted in gray.

| SPs per 2M cut | $\sigma_N^2$, $T_\Omega$ | $1.0 \times 10^{-8}$ | $1.0 \times 10^{-9}$ | $1.0 \times 10^{-10}$ | $1.0 \times 10^{-11}$ |
|---|---|---|---|---|---|
| 0 | MaxD | 9.26 | 0.42 | −0.47 | 1.15 |
| | MinD | 1.47 | −4.14 | −3.21 | −0.73 |
| | RMSD | 6.23 | 1.62 | 1.48 | 0.39 |
| | No. SPs | 8382 | 9690 | 10928 | 12003 |
| 5 | MaxD | 1.93 | −0.92 | 1.29 | 1.31 |
| | MinD | −4.49 | −5.97 | −1.50 | −0.10 |
| | RMSD | 1.37 | 3.24 | 0.64 | 0.30 |
| | No. SPs | 9441 | 10675 | 11881 | 12925 |
| 10 | MaxD | 9.81 | 0.35 | 1.33 | 0.24 |
| | MinD | 2.13 | −4.37 | −0.07 | −0.70 |
| | RMSD | 4.30 | 1.34 | 0.46 | 0.18 |
| | No. SPs | 7630 | 12031 | 13137 | 14211 |
| 15 | MaxD | 5.67 | 1.52 | 1.34 | 0.20 |
| | MinD | −2.12 | −0.30 | −1.27 | −1.38 |
| | RMSD | 2.72 | 0.84 | 0.65 | 0.32 |
| | No. SPs | 6854 | 8484 | 12040 | 15447 |
| 20 | MaxD | 3.48 | 3.52 | −0.17 | 0.21 |
| | MinD | −2.96 | −0.88 | −1.88 | −1.13 |
| | RMSD | 1.84 | 1.09 | 0.79 | 0.27 |
| | No. SPs | 6801 | 8020 | 9835 | 14323 |
| 25 | MaxD | 2.75 | 1.44 | 0.50 | 0.16 |
| | MinD | −4.21 | −0.25 | −2.10 | −0.86 |
| | RMSD | 1.66 | 0.66 | 0.60 | 0.20 |
| | No. SPs | 6749 | 8561 | 9684 | 13979 |
| 30 | MaxD | 2.75 | 1.45 | – | 0.27 |
| | MinD | −4.21 | −0.15 | – | −0.66 |
| | RMSD | 1.66 | 0.61 | – | 0.19 |
| | No. SPs | 6749 | 8570 | – | 13866 |

# S5 Varying ADGA Thresholds in GPR-ADGA Computations: Example of Pyrimidine

Table S12: GPR-ADGA-2M computations for pyrimidine. ADGA criteria used are $\epsilon_{\text{rel}} = 1.0 \times 10^{-2}$, $\epsilon_{\text{abs}} = 1.0 \times 10^{-5}$, and $\epsilon_{\rho} = 1.0 \times 10^{-3}$. Deviations (in $\text{cm}^{-1}$) are calculated with respect to the reference ADGA-2M calculation employing same criteria.

| $\sigma_N^2$, $T_\Omega$ | $1.0 \times 10^{-8}$ | $1.0 \times 10^{-9}$ | $1.0 \times 10^{-10}$ | $1.0 \times 10^{-11}$ | ADGA ref. |
|---|---|---|---|---|---|
| MaxD | 5.67 | 1.52 | 1.34 | 0.20 | – |
| MinD | −2.12 | −0.30 | −1.27 | −1.38 | – |
| RMSD | 2.72 | 0.84 | 0.65 | 0.32 | – |
| No. SPs | 6854 | 8484 | 12040 | 15447 | 16022 |

Table S13: GPR-ADGA-2M computations for pyrimidine. ADGA criteria used are $\epsilon_{\text{rel}} = 1.0 \times 10^{-3}$, $\epsilon_{\text{abs}} = 1.0 \times 10^{-5}$, and $\epsilon_{\rho} = 1.0 \times 10^{-3}$. Deviations (in $\text{cm}^{-1}$) are calculated with respect to the reference ADGA-2M calculation employing same criteria.

| $\sigma_N^2$, $T_\Omega$ | $1.0 \times 10^{-8}$ | $1.0 \times 10^{-9}$ | $1.0 \times 10^{-10}$ | $1.0 \times 10^{-11}$ | ADGA ref. |
|---|---|---|---|---|---|
| MaxD | 7.49 | 2.26 | 1.06 | 0.41 | – |
| MinD | −4.69 | −1.78 | −1.38 | −1.02 | – |
| RMSD | 3.09 | 1.50 | 0.68 | 0.26 | – |
| No. SPs | 6572 | 8060 | 12613 | 16450 | 20756 |

Table S14: GPR-ADGA-2M computations for pyrimidine. ADGA criteria used are $\epsilon_{\text{rel}} = 1.0 \times 10^{-2}$, $\epsilon_{\text{abs}} = 1.0 \times 10^{-6}$, and $\epsilon_{\rho} = 1.0 \times 10^{-3}$. Deviations (in $\text{cm}^{-1}$) are calculated with respect to the reference ADGA-2M calculation employing same criteria.

| $\sigma_N^2$, $T_\Omega$ | $1.0 \times 10^{-8}$ | $1.0 \times 10^{-9}$ | $1.0 \times 10^{-10}$ | $1.0 \times 10^{-11}$ | ADGA ref. |
|---|---|---|---|---|---|
| MaxD | 5.27 | 1.28 | −0.72 | 0.36 | – |
| MinD | −1.17 | −1.04 | −2.66 | −1.17 | – |
| RMSD | 2.72 | 0.69 | 1.67 | 0.28 | – |
| No. SPs | 7960 | 10243 | 13933 | 18833 | 33836 |

# S6 GPR-ADGA Computational Cost

Table S15: CPU and wall times required for GPR-ADGA and reference ADGA computations of ethylene PESs using the HF method. Times spent on SPs, VSCF, polynomial fit of the PES, energy predictions, hyperparameter optimization (denoted as HOPT) are presented. For computational details, see the main text. All values are given in minutes.

| $T_\Omega$, $\sigma_N^2$ | $1.0 \times 10^{-9}$ | | $1.0 \times 10^{-10}$ | | $1.0 \times 10^{-11}$ | | ADGA | |
|---|---|---|---|---|---|---|---|---|
| | CPU | Wall | CPU | Wall | CPU | Wall | CPU | Wall |
| SPs | 0.76 | 9.38 | 0.88 | 10.51 | 0.96 | 11.93 | 1.17 | 21.21 |
| VSCF | 6.32 | 4.83 | 7.39 | 5.34 | 5.00 | 3.96 | 0.26 | 0.20 |
| Fit | 0.21 | 0.10 | 0.23 | 0.08 | 0.24 | 0.06 | 0.01 | 0.01 |
| Pred. | 2.12 | 0.18 | 3.36 | 0.32 | 4.30 | 0.44 | – | – |
| HOPT | 7.04 | 4.55 | 7.21 | 4.38 | 6.68 | 4.35 | – | – |
| Other | 0.78 | 1.63 | 0.90 | 1.26 | 0.86 | 1.05 | 0.15 | 0.10 |
| Total | 17.24 | 20.67 | 19.96 | 21.90 | 18.04 | 21.80 | 1.59 | 21.52 |

Table S16: CPU and wall times required for GPR-ADGA and reference ADGA computations of ethylene PESs using the RI-MP2-F12 method. Times spent on SPs, VSCF, polynomial fit of the PES, energy predictions, hyperparameter optimization (denoted as HOPT) are presented. For computational details, see the main text. All values are given in minutes.

| $T_\Omega$, $\sigma_N^2$ | $1.0 \times 10^{-9}$ | | $1.0 \times 10^{-10}$ | | $1.0 \times 10^{-11}$ | | ADGA | |
|---|---|---|---|---|---|---|---|---|
| | CPU | Wall | CPU | Wall | CPU | Wall | CPU | Wall |
| SPs | 1.05 | 14.95 | 1.21 | 17.12 | 1.40 | 19.17 | 2.03 | 36.91 |
| VSCF | 6.69 | 5.07 | 4.83 | 3.86 | 5.70 | 4.51 | 0.26 | 0.20 |
| Fit | 0.24 | 0.07 | 0.25 | 0.09 | 0.28 | 0.09 | 0.02 | 0.00 |
| Pred. | 3.01 | 0.27 | 3.75 | 0.35 | 6.07 | 0.60 | – | – |
| HOPT | 6.08 | 3.85 | 4.16 | 2.60 | 5.06 | 3.19 | – | – |
| Other | 0.88 | 1.05 | 0.90 | 1.36 | 1.04 | 1.29 | 0.13 | 0.09 |
| Total | 17.95 | 25.25 | 15.10 | 25.38 | 19.56 | 28.85 | 2.43 | 37.21 |

Table S17: CPU and wall times required for GPR-ADGA and reference ADGA computations of ethylene PESs using the CCSD(F12*)(T) method. Times spent on SPs, VSCF, polynomial fit of the PES, energy predictions, hyperparameter optimization (denoted as HOPT) are presented. For computational details, see the main text. All values are given in minutes.

| $T_\Omega$, $\sigma_N^2$ | $1.0 \times 10^{-9}$ | | $1.0 \times 10^{-10}$ | | $1.0 \times 10^{-11}$ | | ADGA | |
|---|---|---|---|---|---|---|---|---|
| | CPU | Wall | CPU | Wall | CPU | Wall | CPU | Wall |
| SPs | 7.57 | 119.25 | 9.06 | 143.88 | 10.38 | 165.81 | 18.95 | 310.08 |
| VSCF | 5.86 | 4.33 | 5.05 | 3.90 | 5.85 | 4.41 | 0.47 | 0.27 |
| Fit | 0.30 | 0.07 | 0.31 | 0.09 | 0.06 | 0.10 | 0.02 | 0.01 |
| Pred. | 2.66 | 0.21 | 4.03 | 0.36 | 5.80 | 0.56 | – | – |
| HOPT | 10.35 | 6.14 | 8.03 | 5.03 | 5.33 | 3.12 | – | – |
| Other | 0.72 | 0.96 | 0.64 | 1.05 | 0.82 | 1.31 | 0.14 | 0.12 |
| Total | 27.46 | 130.96 | 27.12 | 154.31 | 28.24 | 175.31 | 19.58 | 310.48 |

## S7 Vibrational Couple Cluster Computations

Table S18: GPR-ADGA-2M computations for ethylene employing the HF electronic structure and VCC[2] vibrational structure methods. Results for different GPR-ADGA thresholds ($T_\Omega = \sigma_N^2$) are shown. ADGA criteria used are $\epsilon_{\text{rel}} = 1.0 \times 10^{-2}$, $\epsilon_{\text{abs}} = 1.0 \times 10^{-5}$, and $\epsilon_\rho = 1.0 \times 10^{-3}$. Deviations (in $\text{cm}^{-1}$) are calculated with respect to the reference ADGA-2M calculation employing same criteria.

| | $1.0 \times 10^{-9}$ | $1.0 \times 10^{-10}$ | $1.0 \times 10^{-11}$ | ADGA ref. |
|---|---|---|---|---|
| MaxD | 3.93 | 1.79 | 0.00 | – |
| MinD | −0.05 | −0.18 | −0.35 | – |
| RMSD | 1.79 | 0.76 | 0.16 | – |
| No. SPs | 1840 | 2099 | 2393 | 4487 |

Table S19: GPR-ADGA-2M computations for ethylene employing the RI-MP2-F12 electronic structure and VCC[2] vibrational structure methods. Results for different GPR-ADGA thresholds ($T_\Omega = \sigma_N^2$) are shown. ADGA criteria used are $\epsilon_{\text{rel}} = 1.0 \times 10^{-2}$, $\epsilon_{\text{abs}} = 1.0 \times 10^{-5}$, and $\epsilon_\rho = 1.0 \times 10^{-3}$. Deviations (in $\text{cm}^{-1}$) are calculated with respect to the reference ADGA-2M calculation employing same criteria.

| | $1.0 \times 10^{-9}$ | $1.0 \times 10^{-10}$ | $1.0 \times 10^{-11}$ | ADGA ref. |
|---|---|---|---|---|
| MaxD | 8.16 | 4.60 | 2.13 | – |
| MinD | −2.95 | −1.86 | −0.53 | – |
| RMSD | 2.88 | 1.51 | 0.80 | – |
| No. SPs | 1904 | 2174 | 2475 | 5097 |

Table S20: GPR-ADGA-2M computations for ethylene employing the CCSD(F12*)(T) electronic structure and VCC[2] vibrational structure methods. Results for different GPR-ADGA thresholds ($T_\Omega = \sigma_N^2$) are shown. ADGA criteria used are $\epsilon_{\text{rel}} = 1.0 \times 10^{-2}$, $\epsilon_{\text{abs}} = 1.0 \times 10^{-5}$, and $\epsilon_\rho = 1.0 \times 10^{-3}$. Deviations (in $\text{cm}^{-1}$) are calculated with respect to the reference ADGA-2M calculation employing same criteria.

| | $1.0 \times 10^{-9}$ | $1.0 \times 10^{-10}$ | $1.0 \times 10^{-11}$ | ADGA ref. |
|---|---|---|---|---|
| MaxD | 9.24 | 5.13 | 0.23 | – |
| MinD | −0.07 | −1.00 | −0.25 | – |
| RMSD | 3.40 | 1.89 | 0.12 | – |
| No. SPs | 1766 | 2184 | 2503 | 4960 |

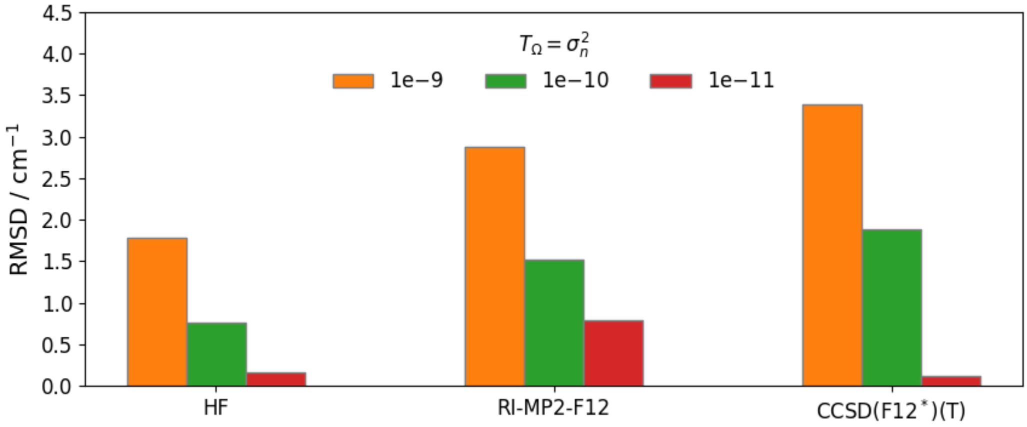


Figure S1: Comparison of 2M PESs calculated for ethylene using GPR-ADGA and reference ADGA. The PESs are computed with the HF, RI-MP2-F12, and CCSD(F12*)(T) electronic structure methods. RMSDs (in cm$^{-1}$) of VCC[2] fundamental frequencies are shown. Results generated with GPR-ADGA criteria $T_\Omega$ and $\sigma_N^2$ being simultaneously varied in the series $1.0 \times 10^{-9}$, $1.0 \times 10^{-10}$, and $1.0 \times 10^{-11}$ are shown in orange, green, and red colors, respectively.

# References


[1] F. Pedregosa, G. Varoquaux, A. Gramfort, V. Michel, B. Thirion, O. Grisel, M. Blondel, P. Prettenhofer, R. Weiss, V. Dubourg, J. Vanderplas, A. Passos, D. Cournapeau, M. Brucher, M. Perrot, É. Duchesnay. Scikit-learn: Machine Learning in Python. *JMLR*, **12** (2011) 2825–2830.

[2] Scikit-learn documentation. `https://scikit-learn.org/stable/modules/generated/sklearn.preprocessing.StandardScaler.html`. Access date: February 8, 2023.

[3] S. Basak, S. Petit, J. Bect, E. Vazquez. Numerical issues in maximum likelihood parameter estimation for gaussian process interpolation. In G. Nicosia, V. Ojha, E. La Malfa, G. La Malfa, G. Jansen, P. M. Pardalos, G. Giuffrida, R. Umeton, Eds., *Machine Learning, Optimization, and Data Science*, p. 116–131, Cham, 2022. Springer International Publishing.

[4] N. Ulapane, K. Thiyagarajan, S. Kodagoda. Hyper-Parameter Initialization for Squared Exponential Kernel-based Gaussian Process Regression. In *2020 15th IEEE Conference on Industrial Electronics and Applications (ICIEA)*, p. 1154–1159, 2020.
